# Supplementary material for: Impact of boron atom clustering on the electronic structure of (B,In)N alloys
Source: arXiv:2401.07623 source file (2024-01-15)
Supplement: Supplementary file 1 [file BInN-SI.pdf]

# Supporting Information: Impact of boron atom clustering on the electronic structure of (B,In)N alloys

Cara-Lena Nies[1] and Stefan Schulz[2,1,*]

[1]Tyndall National Institute, University College Cork, Lee Maltings, Dyke Parade, Cork, T12 R5CP, Ireland

[2]School of Physics, University College Cork, College Road, Cork, Ireland

[*]Corresponding author: stefan.schulz@tyndall.ie

## Contents

**S1: Additional Data for (B,In)N geometries** **2**

**S2: Density of States Data for "line" and "z-line" configurations** **3**

# S1: Additional Data for (B,In)N geometries

| Configuration | BN Content | c-Parameter | Lattice Parameter | | Band Gap (eV) | % Change |
|---|---|---|---|---|---|---|
| | | | a (Å) | c (Å) | | |
| InN | 0 % | 1.315 | 10.7420 | 17.3856 | 0.690 | |
| BN | 100 % | 1.3 | 7.6638 | 12.6732 | 6.699 ($\Gamma - K$) | |
| Single B | 1.9 % | 1.315 | 10.6895 | 17.2825 | 0.690 | 0.02 |
| 2 B z-line | 3.7 % | 1.314 | 10.6723 | 17.2036 | 0.000 | - |
| 2 B apart | 3.7 % | 1.314 | 10.6328 | 17.1932 | 0.693 | 0.50 |
| 2 B line | 3.7 % | 1.314 | 10.6901 | 17.1395 | 0.000 | - |
| 3 B close | 5.6 % | 1.314 | 10.6542 | 17.1166 | 0.000 | - |
| 3 B apart | 5.6 % | 1.314 | 10.5804 | 17.0851 | 0.677 | -1.84 |
| 3 B line | 5.6 % | 1.314 | 10.6513 | 17.0710 | 0.372 | -46.13 |
| 3 B z-line | 5.6 % | 1.314 | 10.6473 | 17.3004 | 0.766 | 10.97 |
| 4 B close | 7.4 % | 1.314 | 10.6065 | 17.0383 | 0.000 | - |
| 4 B apart | 7.4 % | 1.314 | 10.5187 | 16.9920 | 0.703 | 1.85 |
| 4 B line | 7.4 % | 1.314 | 10.6745 | 17.0038 | 0.000 | - |
| 4 B z-line | 7.4 % | 1.314 | 10.4961 | 17.3808 | 0.000 | - |

Table S1: Data for (B,In)N cluster geometries. The percentage change was calculated with respect to the band gap of InN and such that a negative change indicates a decrease in the band gap.

## S2: Densities of States Data for "line" and "z-line" configurations

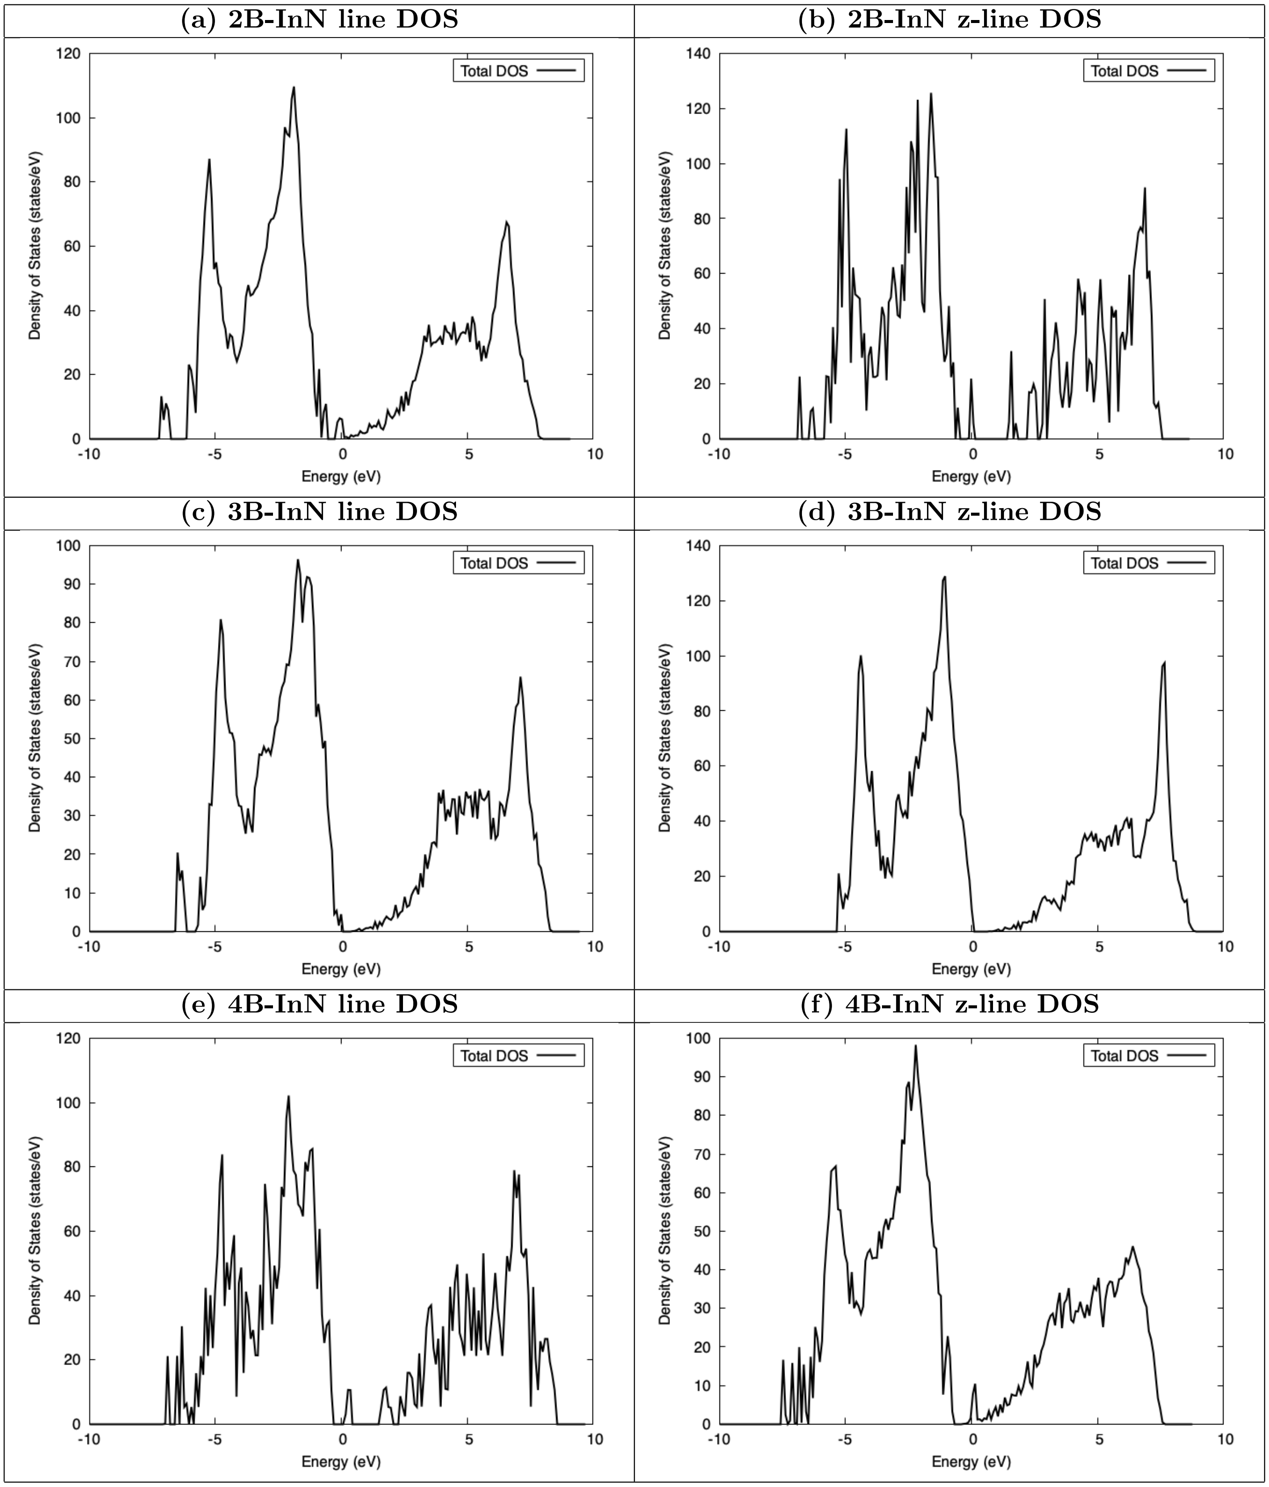


Figure S1: Density of States for line and z-line configurations discussed in the main text of the manuscript.
